# Supplementary material for: SkillCoach: Self-Evolving Rubrics for Evaluating and Enhancing Agentic Skill-Use
Source: arXiv:2607.01874 source file (2026-07-02)
Supplement: Supplementary file 1 [file appendix.tex]

\newpage
\beginappendix

\section{Details of tools}
\label{app:tools}

\noindent \textbf{Search Tools} 
External search is essential for agent systems to extend knowledge boundaries, and we have implemented several fine grain search tools as follows:

\resizebox{0.85\textwidth}{!}{
\begin{promptbox}[Search Tools]{jingdongred}
    \textbf{Web Search}
    \begin{itemize}
    \item \textbf{Google Search}
    \item \textbf{Bing Search}
    \item \textbf{DuckDuckGo Search}
    \item \textbf{Integrated Search}
    \end{itemize}
    \textbf{Github Search}
    \begin{itemize}
        \item \textbf{Repository Search}
        \item \textbf{Issue Search}
        \item \textbf{PR Search}
        \item \textbf{Releases Search}
    \end{itemize}
    \textbf{Arxiv Search}
    \begin{itemize}
        \item \textbf{Advanced Search}
    \end{itemize}
    \textbf{Wiki Search}
    \begin{itemize}
        \item \textbf{Wikipedia Search}
    \end{itemize}      
\end{promptbox}
}

\noindent \textbf{Parsing Tools}
The correct parsing of files is a prerequisite for the Agent system to effectively utilize the information obtained. We have implemented a wealth of parsing tools as follows:

\resizebox{0.85\textwidth}{!}{
\begin{promptbox}[Parsing Tools]{jingdongred}
    \textbf{File Parsing}
    \begin{itemize}
        \item \textbf{PDF Tool} 
        \item \textbf{Doc Tool}
        \item \textbf{Text Tool}
        \item \textbf{Image Tool}
        \item \textbf{OCR Tool}
        \item \textbf{Audio Tool}
        \item \textbf{PDB Tool}
        \item \textbf{HTML Tool}
        \item \textbf{Zip Tool}
    \end{itemize}
    \textbf{Page Parsing}
    \begin{itemize}
        \item \textbf{Webpage Tool}
        \item \textbf{Archived Page Tool}
        \item \textbf{Wiki Page Tool}
        \item \textbf{Youtube Page Tool}
    \end{itemize}
\end{promptbox}
}

\noindent \textbf{Youtube Tools}
Without using the multimodal video mode, we have implemented multiple tools to capture different content of YouTube videos separately:

\newpage
\resizebox{0.85\textwidth}{!}{
\begin{promptbox}[Parsing Tools]{jingdongred}
    \textbf{Fetch Tool}
    \begin{itemize}
        \item \textbf{Video Introduction Tool}
        \item \textbf{Frame Screenshot Tool}
        \item \textbf{Subtitle Tool}
        \item \textbf{Audio Tool}
    \end{itemize}
\end{promptbox}
}

\noindent \textbf{Browswer Tools}
For some tasks that require interaction with web pages, we directly load the mcp tool provided by playwright.
